# Supplementary material for: LIBRE: Learning Interpretable Boolean Rule Ensembles
Source: arXiv:1911.06537 source file (2019-11-15)
Supplement: Supplementary file 1 [file interpretable_rule_sets.tex]

We demonstrated experimentally that \EBRS predictive performances are at least comparable with 
black box models, whereas there is no friendly match with the tested interpretable methods. 
However, we have also noticed that such good performances lead to rule sets that are slightly less interpretable than \RIPPERK and \BRS. 
Here, we show that it is possible to sacrifice a bit of predictive 
performances to gain interpretability.

\begin{figure}[ht]
    \centering
    \caption{Interpretable rulesets for 10 datasets.}
    \label{fig:interpretable_rulesets}
    \begin{subfigure}[b]{0.4\textwidth}
        \includegraphics[width=\textwidth]{images/adult.pdf}
        \caption{\Adult}
        \label{fig:interpretable_adult}
    \end{subfigure}
    \begin{subfigure}[b]{0.4\textwidth}
        \includegraphics[width=\textwidth]{images/australian.pdf}
        \caption{\Australian}
        \label{fig:interpretable_australian}
    \end{subfigure}
    \begin{subfigure}[b]{0.4\textwidth}
        \includegraphics[width=\textwidth]{images/bank.pdf}
        \caption{\Bank}
        \label{fig:interpretable_bank}
    \end{subfigure}
    \begin{subfigure}[b]{0.4\textwidth}
        \includegraphics[width=\textwidth]{images/heart.pdf}
        \caption{\Heart}
        \label{fig:interpretable_heart}
    \end{subfigure}
    \begin{subfigure}[b]{0.4\textwidth}
        \includegraphics[width=\textwidth]{images/ilpd.pdf}
        \caption{\Ilpd}
        \label{fig:interpretable_ilpd}
    \end{subfigure}
    \begin{subfigure}[b]{0.4\textwidth}
        \includegraphics[width=\textwidth]{images/liver.pdf}
        \caption{\Liver}
        \label{fig:interpretable_liver}
    \end{subfigure}
    \begin{subfigure}[b]{0.4\textwidth}
        \includegraphics[width=\textwidth]{images/pima.pdf}
        \caption{\Pima}
        \label{fig:interpretable_pima}
    \end{subfigure}
    \begin{subfigure}[b]{0.4\textwidth}
        \includegraphics[width=\textwidth]{images/sonar.pdf}
        \caption{\Sonar}
        \label{fig:interpretable_sonar}
    \end{subfigure}
    \begin{subfigure}[b]{0.4\textwidth}
        \includegraphics[width=\textwidth]{images/tictactoe.pdf}
        \caption{\Tictactoe}
        \label{fig:interpretable_tictactoe}
    \end{subfigure}
    \begin{subfigure}[b]{0.4\textwidth}
        \includegraphics[width=\textwidth]{images/transfusion.pdf}
        \caption{\Transfusion}
        \label{fig:interpretable_transfusion}
    \end{subfigure}
\end{figure}
