# Supplementary material for: LIBRE: Learning Interpretable Boolean Rule Ensembles
Source: arXiv:1911.06537 source file (2019-11-15)
Supplement: Supplementary file 2 [file supplement.tex]

\relax
%File: formatting-instruction.tex
\documentclass[letterpaper]{article} % DO NOT CHANGE THIS
\usepackage{aaai19}  % DO NOT CHANGE THIS
\usepackage{times}  % DO NOT CHANGE THIS
\usepackage{helvet} % DO NOT CHANGE THIS
\usepackage{courier}  % DO NOT CHANGE THIS
\usepackage[hyphens]{url}  % DO NOT CHANGE THIS
\usepackage{graphicx} % DO NOT CHANGE THIS
\urlstyle{rm} % DO NOT CHANGE THIS
  % DO NOT CHANGE THIS
\usepackage{graphicx}  % DO NOT CHANGE THIS
\frenchspacing  % DO NOT CHANGE THIS
\setlength{\pdfpagewidth}{8.5in}  % DO NOT CHANGE THIS
\setlength{\pdfpageheight}{11in}  % DO NOT CHANGE THIS

\usepackage{microtype}
\usepackage{booktabs}
\usepackage[linesnumbered,ruled]{algorithm2e}
\usepackage{amsmath}
\usepackage{amssymb}
\usepackage{xspace}
\usepackage{subcaption}
\usepackage{tikz}
\usepackage{rotating}
\usepackage{cleveref}

\usepackage{color}

\input{notation}

%PDF Info Is REQUIRED.
% For /Author, add all authors within the parentheses, separated by commas. No accents or commands.
% For /Title, add Title in Mixed Case. No accents or commands. Retain the parentheses.
 \pdfinfo{
%/Title (Learning Ensembles of Monotone Boolean Functions for Interpretable Classification)
/Title (Supplementary Material for "INTER: An Interpretable Ensemble of Boolean Rules")
/Author (Graziano Mita, Paolo Papotti, Maurizio Filippone, Pietro Michiardi)
} %Leave this	

\setcounter{secnumdepth}{0} %May be changed to 1 or 2 if section numbers are desired.

% The file aaai19.sty is the style file for AAAI Press 
% proceedings, working notes, and technical reports.
%
\setlength\titlebox{2.5in} % If your paper contains an overfull \vbox too high warning at the beginning of the document, use this
% command to correct it. You may not alter the value below 2.5 in
%\title{Learning Ensembles of Monotone Boolean Functions for Interpretable Classification}
\title{Supplementary Material for the paper \\ \INTER: An Interpretable Ensemble of Boolean Rules}
%Your title must be in mixed case, not sentence case. 
% That means all verbs (including short verbs like be, is, using,and go), 
% nouns, adverbs, adjectives should be capitalized, including both words in hyphenated terms, while
% articles, conjunctions, and prepositions are lower case unless they
% directly follow a colon or long dash

%\author{Written by AAAI Press Staff\textsuperscript{\rm 1}\thanks{Primarily Mike Hamilton of the Live Oak Press, LLC, with help from the AAAI Publications Committee}\\ \Large \textbf{AAAI Style Contributions by Pater Patel Schneider,} \\ \Large \textbf{Sunil Issar, J. Scott Penberthy, George Ferguson, Hans Guesgen}\\ % All authors must be in the same font size and format. Use \Large and \textbf to achieve this result when breaking a line
%\textsuperscript{\rm 1}Association for the Advancement of Artificial Intelligence\\ %If you have multiple authors and multiple affiliations
% use superscripts in text and roman font to identify them. For example, Sunil Issar,\textsuperscript{\rm 2} J. Scott Penberthy\textsuperscript{\rm 3} George Ferguson,\textsuperscript{\rm 4} Hans Guesgen\textsuperscript{\rm 5}. Note that the comma should be placed BEFORE the superscript for optimum readability

%\author{Graziano Mita, Paolo Papotti, Maurizio Filippone, Pietro Michiardi\\
%EURECOM, France\\
%name.surname@eurecom.fr}
\begin{document}

\maketitle

\onecolumn

\appendix

\section{Walkthrough Example of the Base Method}
\label{sec:walkthrough_example}
\input{appendix/example}

\section{Parallel and Distributed Implementation}
\label{sec:parallel_and_distributed}
\input{appendix/parallel_and_distributed}

\section{Scalability Experiments}
\label{sec:scalability}
\input{appendix/scalability}

%\section{Performance-Interpretability tradeoff}
%\label{sec:performance-interpretability_tradeoff}
%\input{appendix/performance-interpretability_tradeoff}
%
%\section{Full results}
%\label{sec:full_results}
%\input{appendix/full_results}
%
%\section{Interpretable rule sets}
%\label{sec:interpretable_rule_sets}
%\input{appendix/interpretable_rule_sets}

\clearpage
\bibliographystyle{aaai}
\bibliography{eurecomDS}

\end{document}
